# Supplementary material for: Functional Dynamical Structures in Complex Systems: an Information-Theoretic Approach
Source: arXiv:1703.01878 source file (2017-02-13)
Supplement: Supplementary file 1 [file 7_Appendices.tex]

\begin{appendix}
\chapter{Mathematical Notation}

\end{appendix}
